# Supplementary material for: Recurrent Neural Networks for Multivariate Time Series with Missing Values
Source: arXiv:1606.01865 source file (2016-11-07)
Supplement: Supplementary file 1 [file supplementary-dataprocessing.tex]

In this section we describe the preprocessing details for MIMIC-III dataset\footnote{\url{https://mimic.physionet.org/}}. MIMIC-III provides several relational database tables containing information of data relating to patients who stayed within the intensive care units (ICUs) at Beth Israel Deaconess Medical Center. The admission table contains over 58,000 hospital admission records of 38,645 adults and 7,875 neonates. We chose four tables namely \textit{input events-mv} (fluids into patient, e.g. insulin), \textit{output events} (fluids out of the patient, e.g. urine), \textit{lab events} (lab test results, e,g. pH, Platelet count) and \textit{prescription events} (drugs prescribed by doctors, e.g. aspirin and potassium chloride) to collect the patient data recorded in critical care units and hospital record systems. The inputevents-mv table collects the intake for patients monitored using the iMDSoft Metavision system, in which the data collection and organization is much neater than the earlier Philips CareVue system during 2001-2008.

For our work, we use 19714 admission records collected during 2008-2012 by Metavision data management system which is still employed at the hospital.  From each of the four tables, we chose the top 50 items (i.e. features/variables) since these items are present in many of the patients' records. To avoid/reduce ambiguity and noisy observations, we ensured that all the measurements for a particular variable has only one unit of measurement. We also aggregated the multiple readings of a feature at a single time stamp based on the feature type. For instance, some inputevents features should be averaged while others need to be summed up. This resulted in 99 variables being extracted from the four tables for 19714 patient admission records. The entire variable list is shown in Table~\ref{tab:feature-list}.

\begin{table}[hbt]
\caption{List of extracted features after preprocessing MIMIC-III dataset.}
\label{tab:feature-list}
\vspace{-0.1in}
\small
\begin{center}
\begin{tabular}{ccp{0.64\linewidth}}
\toprule
\textbf{Table Name} & \textbf{Variable IDs} & \multicolumn{1}{c}{\textbf{Variable Names}} \\ \midrule
Output & $1-15$ & Gastric Gastric Tube, Stool Out Stool, Urine Out Incontinent, Ultrafiltrate Ultrafiltrate, Foley, Void, Condom Cath, Fecal Bag, Ostomy (Output), Chest Tube \#1, Chest Tube \#2, Jackson Pratt \#1, OR EBL, Pre-Admission, TF Residual \\ \midrule
Input & $16-48$ & Albumin 5\%, Dextrose 5\%, Fresh Frozen Plasma, Lorazepam (Ativan), Calcium Gluconate, Midazolam (Versed), Phenylephrine, Furosemide (Lasix), Hydralazine, Norepinephrine, Magnesium Sulfate, Nitroglycerin, Insulin - Regular, Insulin - Glargine, Insulin - Humalog, Heparin Sodium, Morphine Sulfate, Potassium Chloride, Packed Red Blood Cells, Gastric Meds, D5 1/2NS, LR, K Phos, Solution, Sterile Water, Metoprolol, Piggyback, OR Crystalloid Intake, OR Cell Saver Intake, PO Intake, GT Flush, KCL (Bolus), Magnesium Sulfate (Bolus) \\ \midrule
Lab Test & $49-89$ & Hematocrit, White Blood Cells, Platelet Count, Hemoglobin, MCHC, MCH, MCV, Red Blood Cells, RDW, Potassium, Sodium, Chloride, Bicarbonate, Anion Gap, Urea Nitrogen, Creatinine, Glucose, Magnesium, Calcium, Total, Phosphate, INR(PT), PT, PTT, Lymphocytes, Monocytes, Neutrophils, Basophils, Eosinophils, Bilirubin, Total, PH, Base Excess, Calculated Total CO2, PO2, PCO2, PH, Specific Gravity, Lactate, Alanine Aminotransferase (ALT), Asparate Aminotransferase (AST), Alkaline Phosphatase, Albumin \\ \midrule
Prescription & $90-99$ & Aspirin, Bisacodyl, Docusate Sodium, D5W, Humulin-R Insulin, Potassium Chloride, Magnesium Sulfate, Metoprolol Tartrate, Sodium Chloride 0.9\% Flush, Pantoprazole \\
\bottomrule
\end{tabular}
\end{center}
\end{table}

For each of the admission records, we collected both the variable value $ x_t $ and the time-stamp of observation $ s_t $. In addition, for each admission record we queried the database tables to get the ICD-9 diagnosis codes. One admission record can be associated with multiple ICD-9 codes. We also queried the discharge time and death time from the Admissions table of MIMIC-III to find the mortality label for each admission record. The ICD-9 diagnosis codes were grouped into 20 categories, shown in Table~\ref{tab:icd9-category}, according to the information from the Thomson Reuters webpage\footnote{\url{http://tdrdata.com/ipd/ipd_SearchForICD9CodesAndDescriptions.aspx}}. The class distribution of the ICD-9 codes is shown in Figure~\ref{fig:mimic3_class_distribution}.

\begin{table}[tbh]
\caption{MIMIC-III ICD-9 diagnosis code category descriptions.}
\label{tab:icd9-category}
\small
\begin{center}
\begin{tabular}{c c c}
  \toprule
  \textbf{Category ID} & \textbf{ICD-9 Codes} & \textbf{Diagnosis Category Name} \\ \midrule
  1 & 001 - 139 & Infectious and Parasitic Diseases \\ \midrule
  2 & 140 - 239 & Neoplasms \\ \midrule
  3 & 240 - 279 & Endocrine, Nutritional, Metabolic, Immunity \\ \midrule
  4 & 280 - 289 & Blood and Blood-Forming Organs \\ \midrule
  5 & 290 - 319 & Mental Disorders \\ \midrule
  6 & 320 - 389 & Nervous System and Sense Organs \\ \midrule
  7 & 390 - 459 & Circulatory System \\ \midrule
  8 & 460 - 519 & Respiratory System \\ \midrule
  9 & 520 - 579 & Digestive System \\ \midrule
  10 & 580 - 629 & Genitourinary System \\ \midrule
  11 & 630 - 677 & Pregnancy, Childbirth, and the Puerperium \\ \midrule
  12 & 680 - 709 & Skin and Subcutaneous Tissue \\ \midrule
  13 & 710 - 739 & Musculoskeletal System and Connective Tissue \\ \midrule
  14 & 740 - 759 & Congenital Anomalies \\ \midrule
  15 & 780 - 789 & Symptoms \\ \midrule
  16 & 790 - 796 & Nonspecific Abnormal Findings \\ \midrule
  17 & 797 - 799 & Ill-defined and Unknown Causes of Morbidity and Mortality \\ \midrule
  18 & 800 - 999 & Injury and Poisoning \\ \midrule
  19 & V Codes & Supplemental V-Codes \\ \midrule
  20 & E Codes & Supplemental E-Codes \\ \bottomrule
\end{tabular}
\end{center}
\end{table}

\begin{figure}[tbh]
\begin{center}
\includegraphics[width=0.45\linewidth]{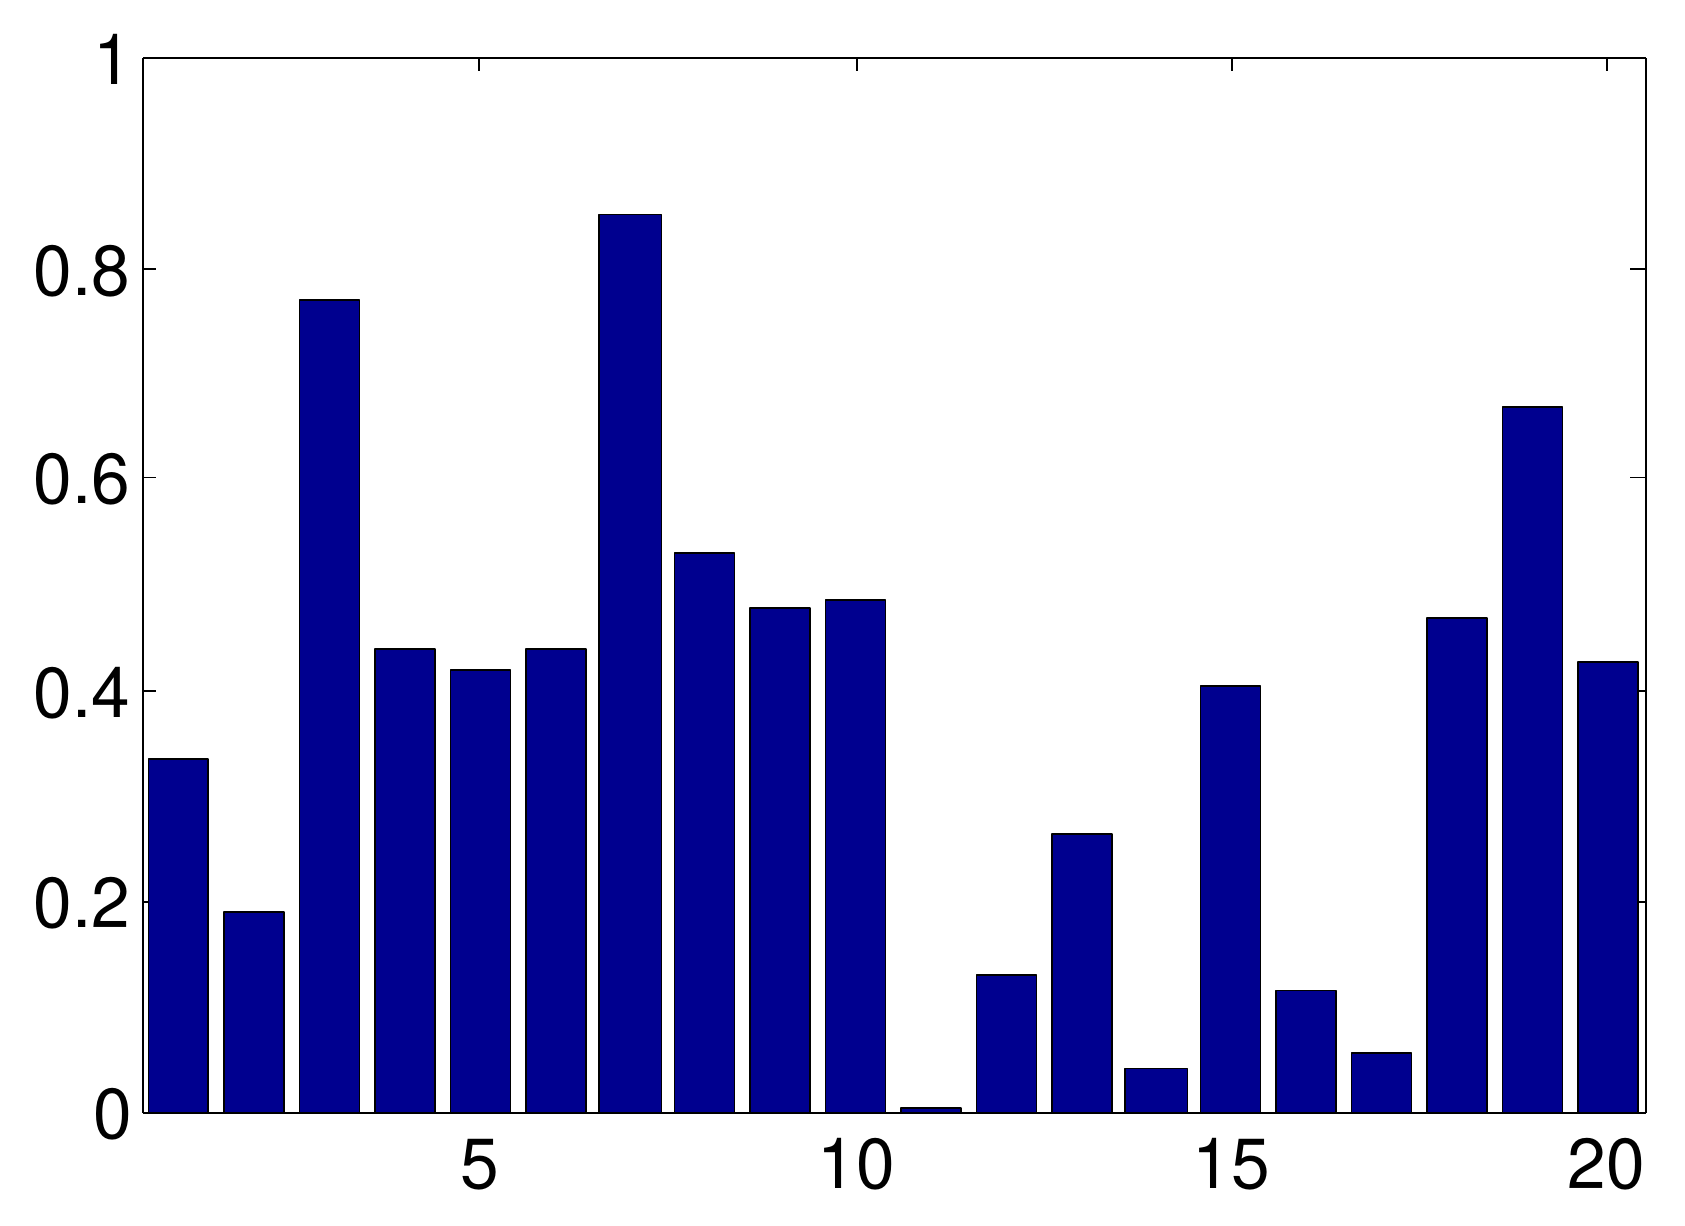}
\end{center}
\vspace{-0.1in}
\caption{\label{fig:mimic3_class_distribution} MIMIC-III ICD-9 diagnosis code class (category) distribution. x-axis, ICD-9 diagnosis category id; y-axis, the ratio of admission records with the diagnosis code.}
\end{figure}
